# Supplementary material for: Observation of anisotropic dispersive dark exciton dynamics in CrSBr
Source: arXiv:2501.06372 source file (2025-08-31)
Supplement: Supplementary file 1 [file supplementary_information.tex]

\documentclass[
 reprint,
superscriptaddress,
onecolumn,
notitlepage,
%groupedaddress,
%unsortedaddress,
%runinaddress,
%frontmatterverbose, 
%preprint,
%showpacs,preprintnumbers,
%nofootinbib,
%nobibnotes,
%bibnotes,
 amsmath,amssymb,
 aps,
%pra,
%prb,
%rmp,
%prstab,
%prstper,
%floatfix,
]{revtex4-2}
\usepackage[no-test-for-array]{nicematrix}
\usepackage{graphicx}% Include figure files
\usepackage{dcolumn}
\usepackage{bm}% bold math
\usepackage{hyperref}% add hypertext capabilities
\usepackage{color}
\usepackage{glossaries}
\usepackage{orcidlink}

%\newcolumntype{C}[1]{>{\Centering}m{#1}}

% Abbreviations here
\newacronym{RIXS}{RIXS}{resonant inelastic x-ray scattering}
\newacronym{XAS}{XAS}{X-ray absorption spectrum}
\newacronym{FWHM}{FWHM}{full-width at half-maximum}
\newacronym{SOC}{SOC}{spin-orbit coupling}
\newacronym{DFT}{DFT}{density functional theory}
\newacronym{AIM}{AIM}{Anderson impurity model}
\newacronym{TFY}{TFY}{total fluorescence yield}

\begin{document}

\title{Observation of anisotropic dispersive dark exciton dynamics in CrSBr}

\author{J. Sears\,\orcidlink{0000-0001-6524-8953}}
\affiliation{Department of Condensed Matter Physics and Materials Science, Brookhaven National Laboratory, Upton, New York 11973, USA}
\author{B. Zager\,\orcidlink{0000-0001-7436-4040}}
\affiliation{National Synchrotron Light Source II, Brookhaven National Laboratory, Upton, New York 11973, USA}
\author{W. He\,\orcidlink{0000-0003-3522-3899}}
\altaffiliation[Current address: ]{Stanford Institute for Materials and Energy Sciences, SLAC National Accelerator Laboratory, Menlo Park, CA 94025}
\affiliation{Department of Condensed Matter Physics and Materials Science, Brookhaven National Laboratory, Upton, New York 11973, USA}
\author{C. A. Occhialini\,\orcidlink{0000-0002-2133-5155}}
\affiliation{National Synchrotron Light Source II, Brookhaven National Laboratory, Upton, New York 11973, USA}
\affiliation{Department of Physics, Columbia University, New York, NY, USA}
\author{Y. Shen\,\orcidlink{0000-0003-4697-4719}}
\altaffiliation[Current address: ]{Beijing National Laboratory for Condensed Matter Physics, Institute of Physics, Chinese Academy of Sciences, Beijing 100190, China; School of Physical Sciences, University of Chinese Academy of Sciences, Beijing 100049,
China}
\author{M. Lajer,\orcidlink{0000-0002-1168-8598}}
\affiliation{Department of Condensed Matter Physics and Materials Science, Brookhaven National Laboratory, Upton, New York 11973, USA}

\author{J. W. Villanova\,\orcidlink{0000-0003-1595-3851}}
\altaffiliation[Current address: ]{Department of Physics and Astronomy, Middle Tennessee State University, Murfreesboro, Tennessee 37132, USA}
\author{T. Berlijn\,\orcidlink{0000-0002-1001-2238}}
\affiliation{Center for Nanophase Materials Sciences, Oak Ridge National Laboratory, Oak Ridge, Tennessee 37831, USA}

\author{F. Yakhou-Harris\,\orcidlink{0000-0002-6798-2286}}
\author{N. B. Brookes\,\orcidlink{0000-0002-1342-9530}}
\affiliation{European Synchrotron Radiation Facility (ESRF), B.P. 220, F-38043 Grenoble Cedex, France}

\author{D.~G.~Chica\,\orcidlink{0000-0001-8616-9365}}
\author{X. Roy\,\orcidlink{0000-0002-8850-0725}}
\affiliation{Chemistry Department, Columbia University, New York, NY 10027, USA}

\author{E. Baldini\,\orcidlink{0000-0002-8131-9974}}
\affiliation{Department of Physics, The University of Texas at Austin, Austin, Texas, USA, 78712}

\author{J. Pelliciari\,\orcidlink{0000-0003-1508-7746}}
\author{V. Bisogni\,\orcidlink{0000-0002-7399-9930}}
\affiliation{National Synchrotron Light Source II, Brookhaven National Laboratory, Upton, New York 11973, USA}

\author{S.~Johnston\,\orcidlink{0000-0002-2343-0113}}
\affiliation{Department of Physics and Astronomy, The University of Tennessee, Knoxville, Tennessee 37966, USA\looseness=-1}
\affiliation{Institute of Advanced Materials and Manufacturing, The University of Tennessee, Knoxville, Tennessee 37996, USA\looseness=-1}

\author{M. Mitrano\,\orcidlink{0000-0002-0102-0391}}
\affiliation{Department of Physics, Harvard University, Cambridge, Massachusetts 02138, USA\looseness=-1}

\author{M. P. M. Dean\,\orcidlink{/0000-0001-5139-3543}}
\email{mdean@bnl.gov}
\affiliation{Department of Condensed Matter Physics and Materials Science, Brookhaven National Laboratory, Upton, New York 11973, USA}

\renewcommand{\thefigure}{S\arabic{figure}}
\renewcommand{\thetable}{S\arabic{table}}

\maketitle

\tableofcontents

\section{Crystal growth of C\MakeLowercase{r}SB\MakeLowercase{r}}
Single crystals of CrSBr were synthesized via chemical vapor transport \cite{Scheie2022spin}. A slightly off-stoichiometric amount of chromium powder, chromium(III) bromide chunks, and sulfur pieces were loaded into a 12.7~mm outer diameter and 10.5~mm inner diameter fused silica tube and sealed to a length of 20~cm under vacuum ($\sim30$~mtorr). The ampule was subjected to a temperature gradient of 950$^\circ$C (source side) to 850$^\circ$C (sink side) for 72 hours in a computer-controlled two-zone tube furnace. The crystals were washed using a Cr$^{2+}$ aqueous solution, deionized water, toluene, and acetone, resulting in shiny black plate-like single crystals with the surface normal along the crystallographic $c$ axis. The crystal morphology tends to be rectangular, with the larger dimension parallel to the $a$ axis. The single crystal used for this measurement had dimensions 1~mm along the $b$ direction and 4~mm along the $a$ direction. The crystal orientation was verified by Laue and single crystal diffraction prior to the \gls*{RIXS} experiment.

\section{Exciton dispersion fitting}
The spectra in Fig.~3 of the main text, were fit with either 5 or 6 Gaussian functions, depending on whether the low-energy exciton was visible. In the $0KL$ plane, the position and width of the excitation at $\sim$1.6~eV were fixed to the fitted value from the scan at low $K$. The full width of the exciton at $\sim$1.37~eV was fixed to the experimental resolution of 30~meV. 

\begin{figure*}[htb!]
    \centering
    \includegraphics[width=0.9\textwidth]{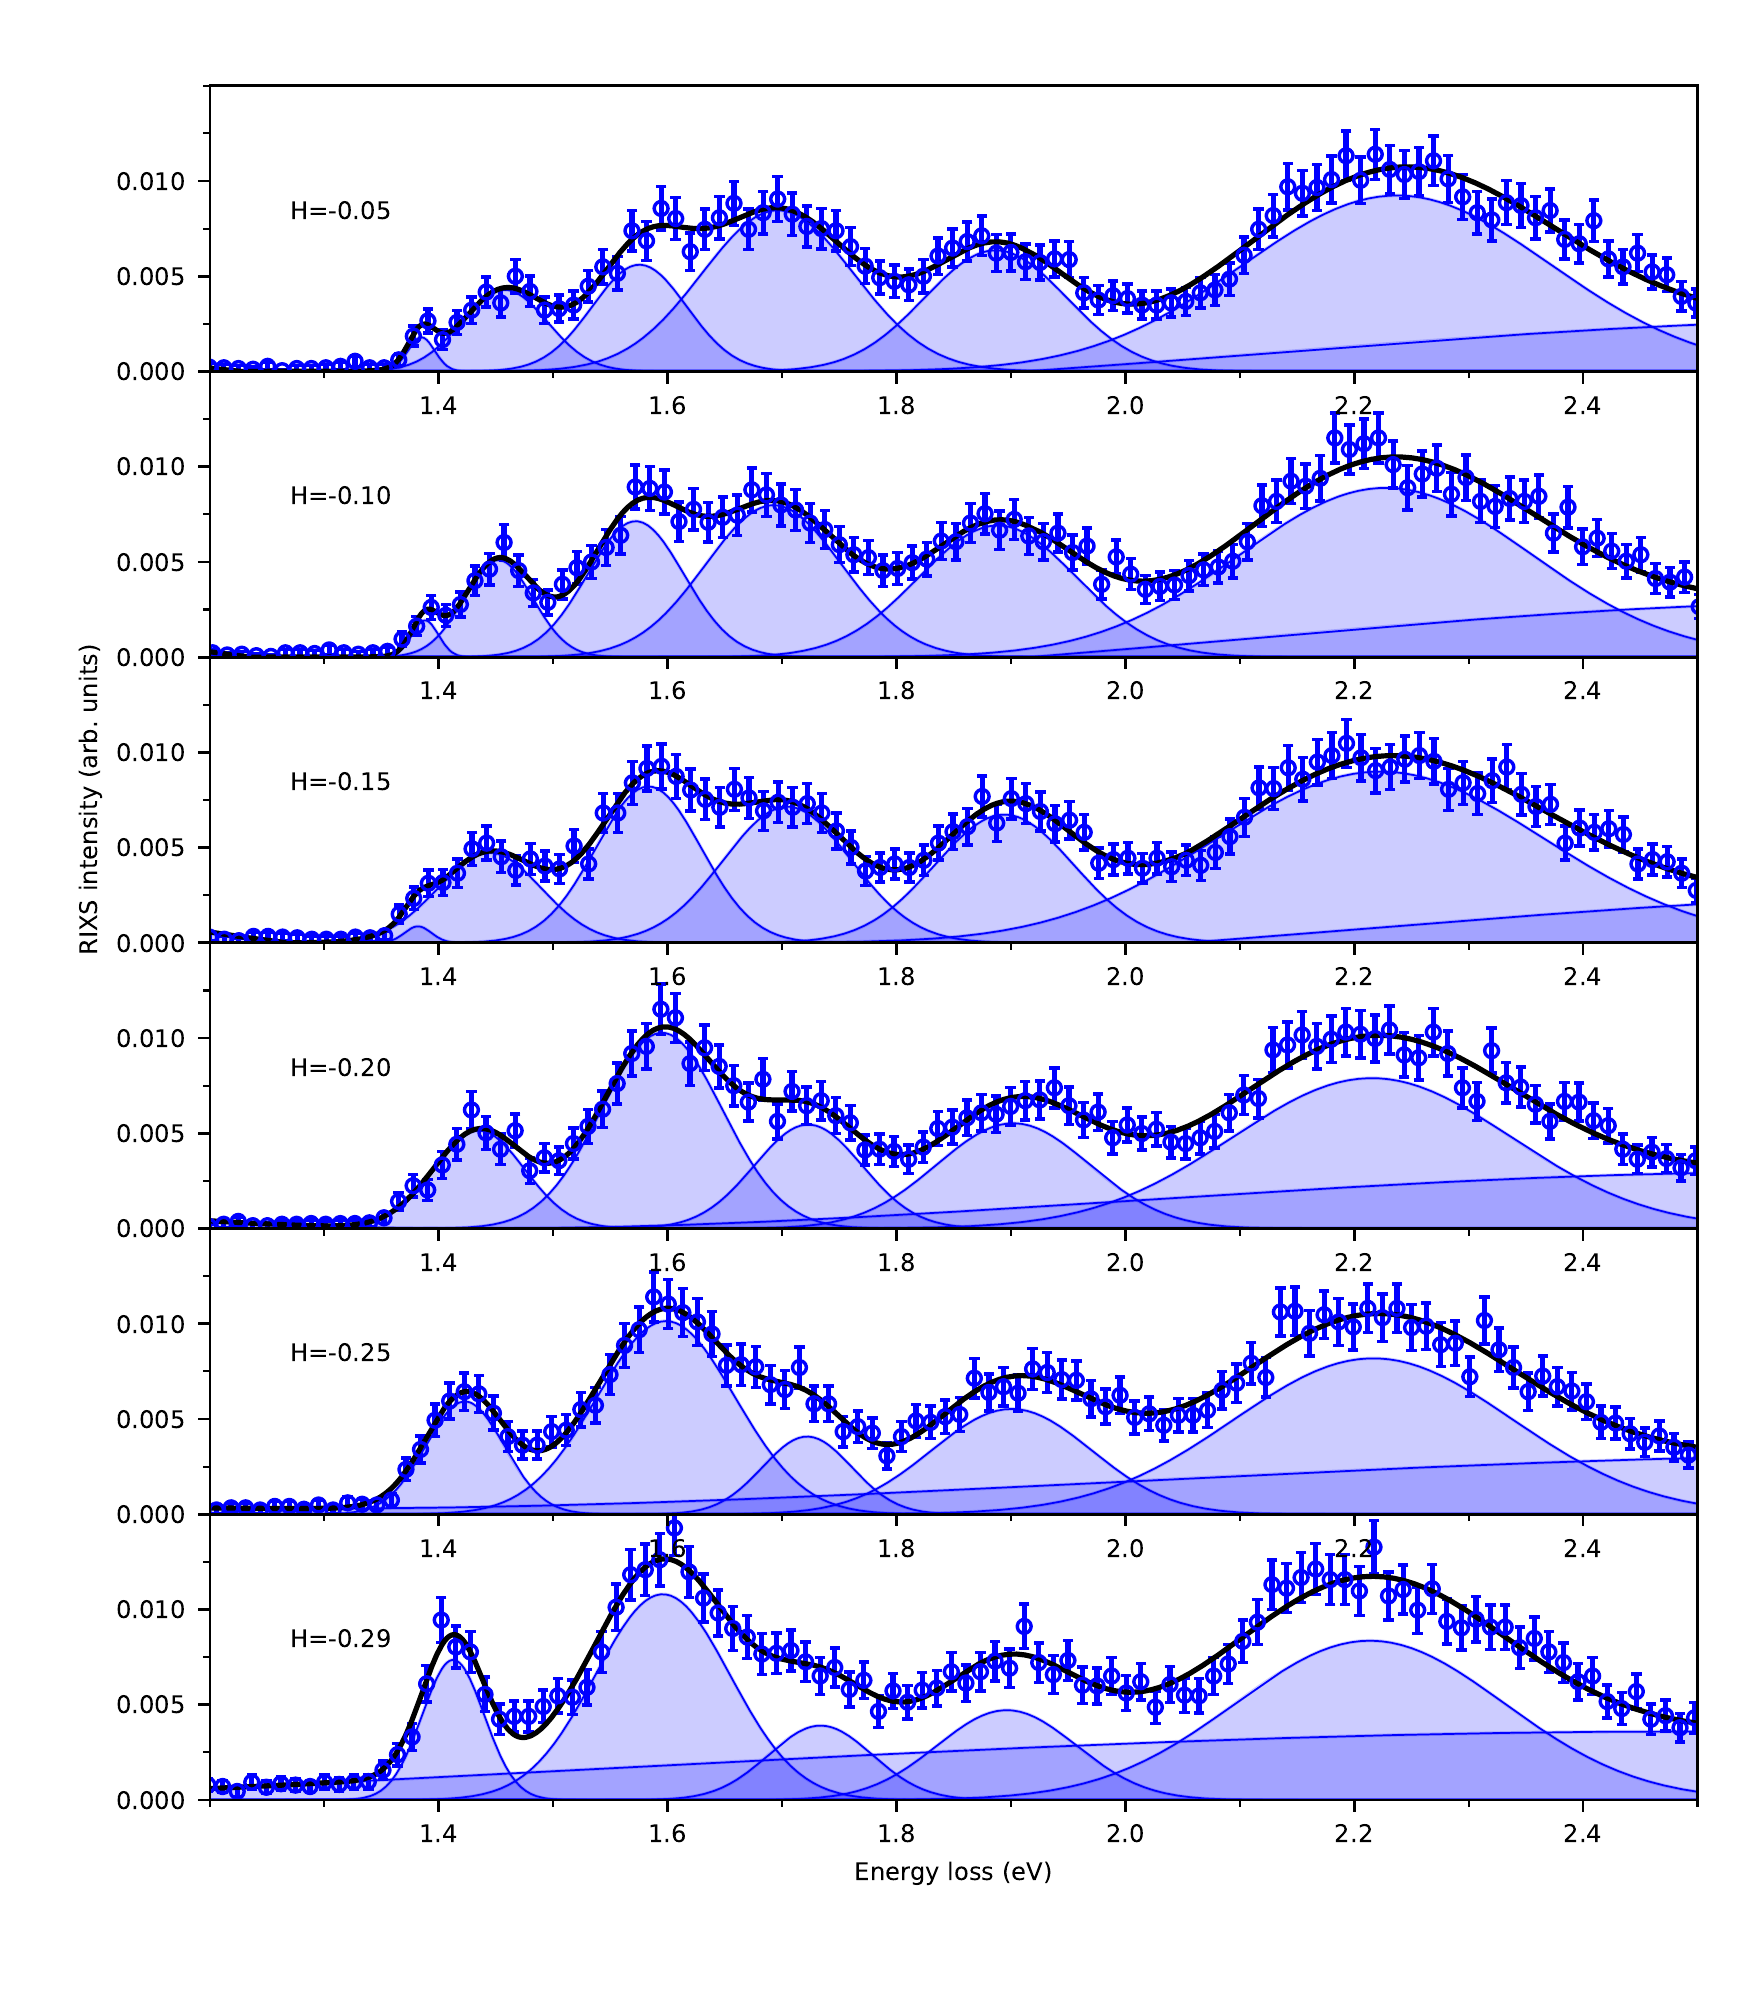}
    \caption{Fits to the spectra in the $H0L$ plane.}
    \label{fig:fits1}
\end{figure*}

\begin{figure*}[htb!]
    \centering
    \includegraphics[width=0.9\textwidth]{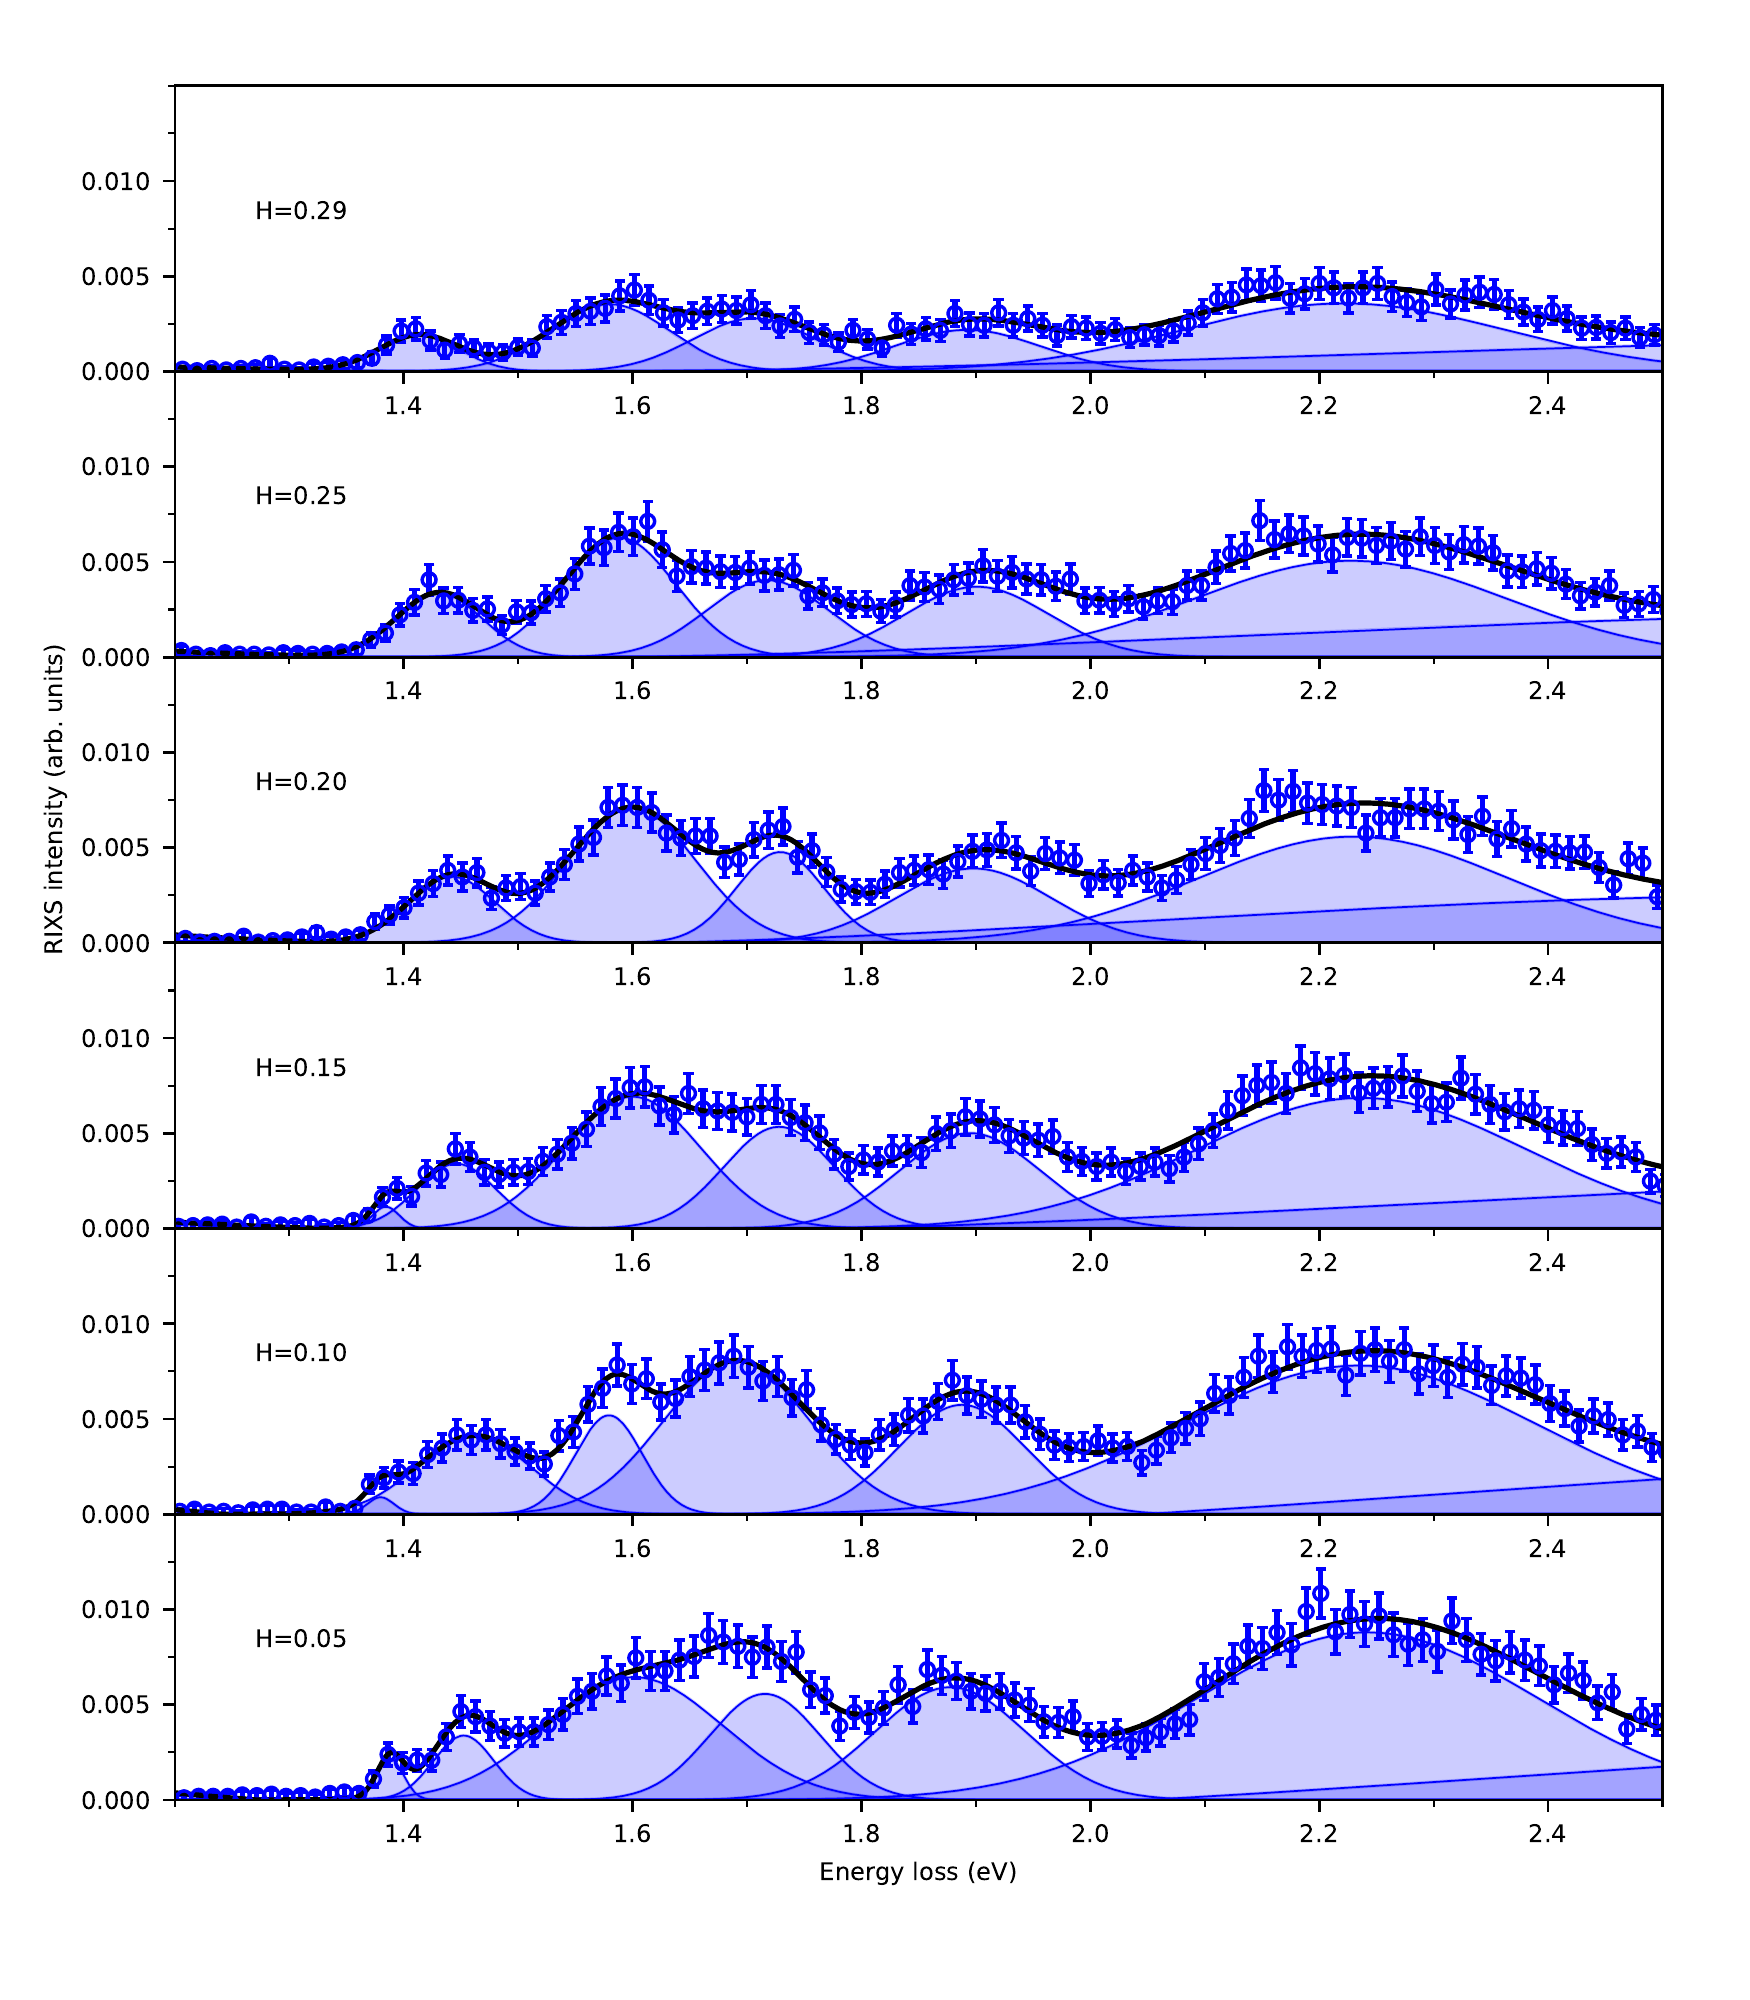}
    \caption{Fits to the spectra in the $H0L$ plane.}
    \label{fig:fits1}
\end{figure*}

\begin{figure*}[htb!]
    \centering
    \includegraphics[width=0.9\textwidth]{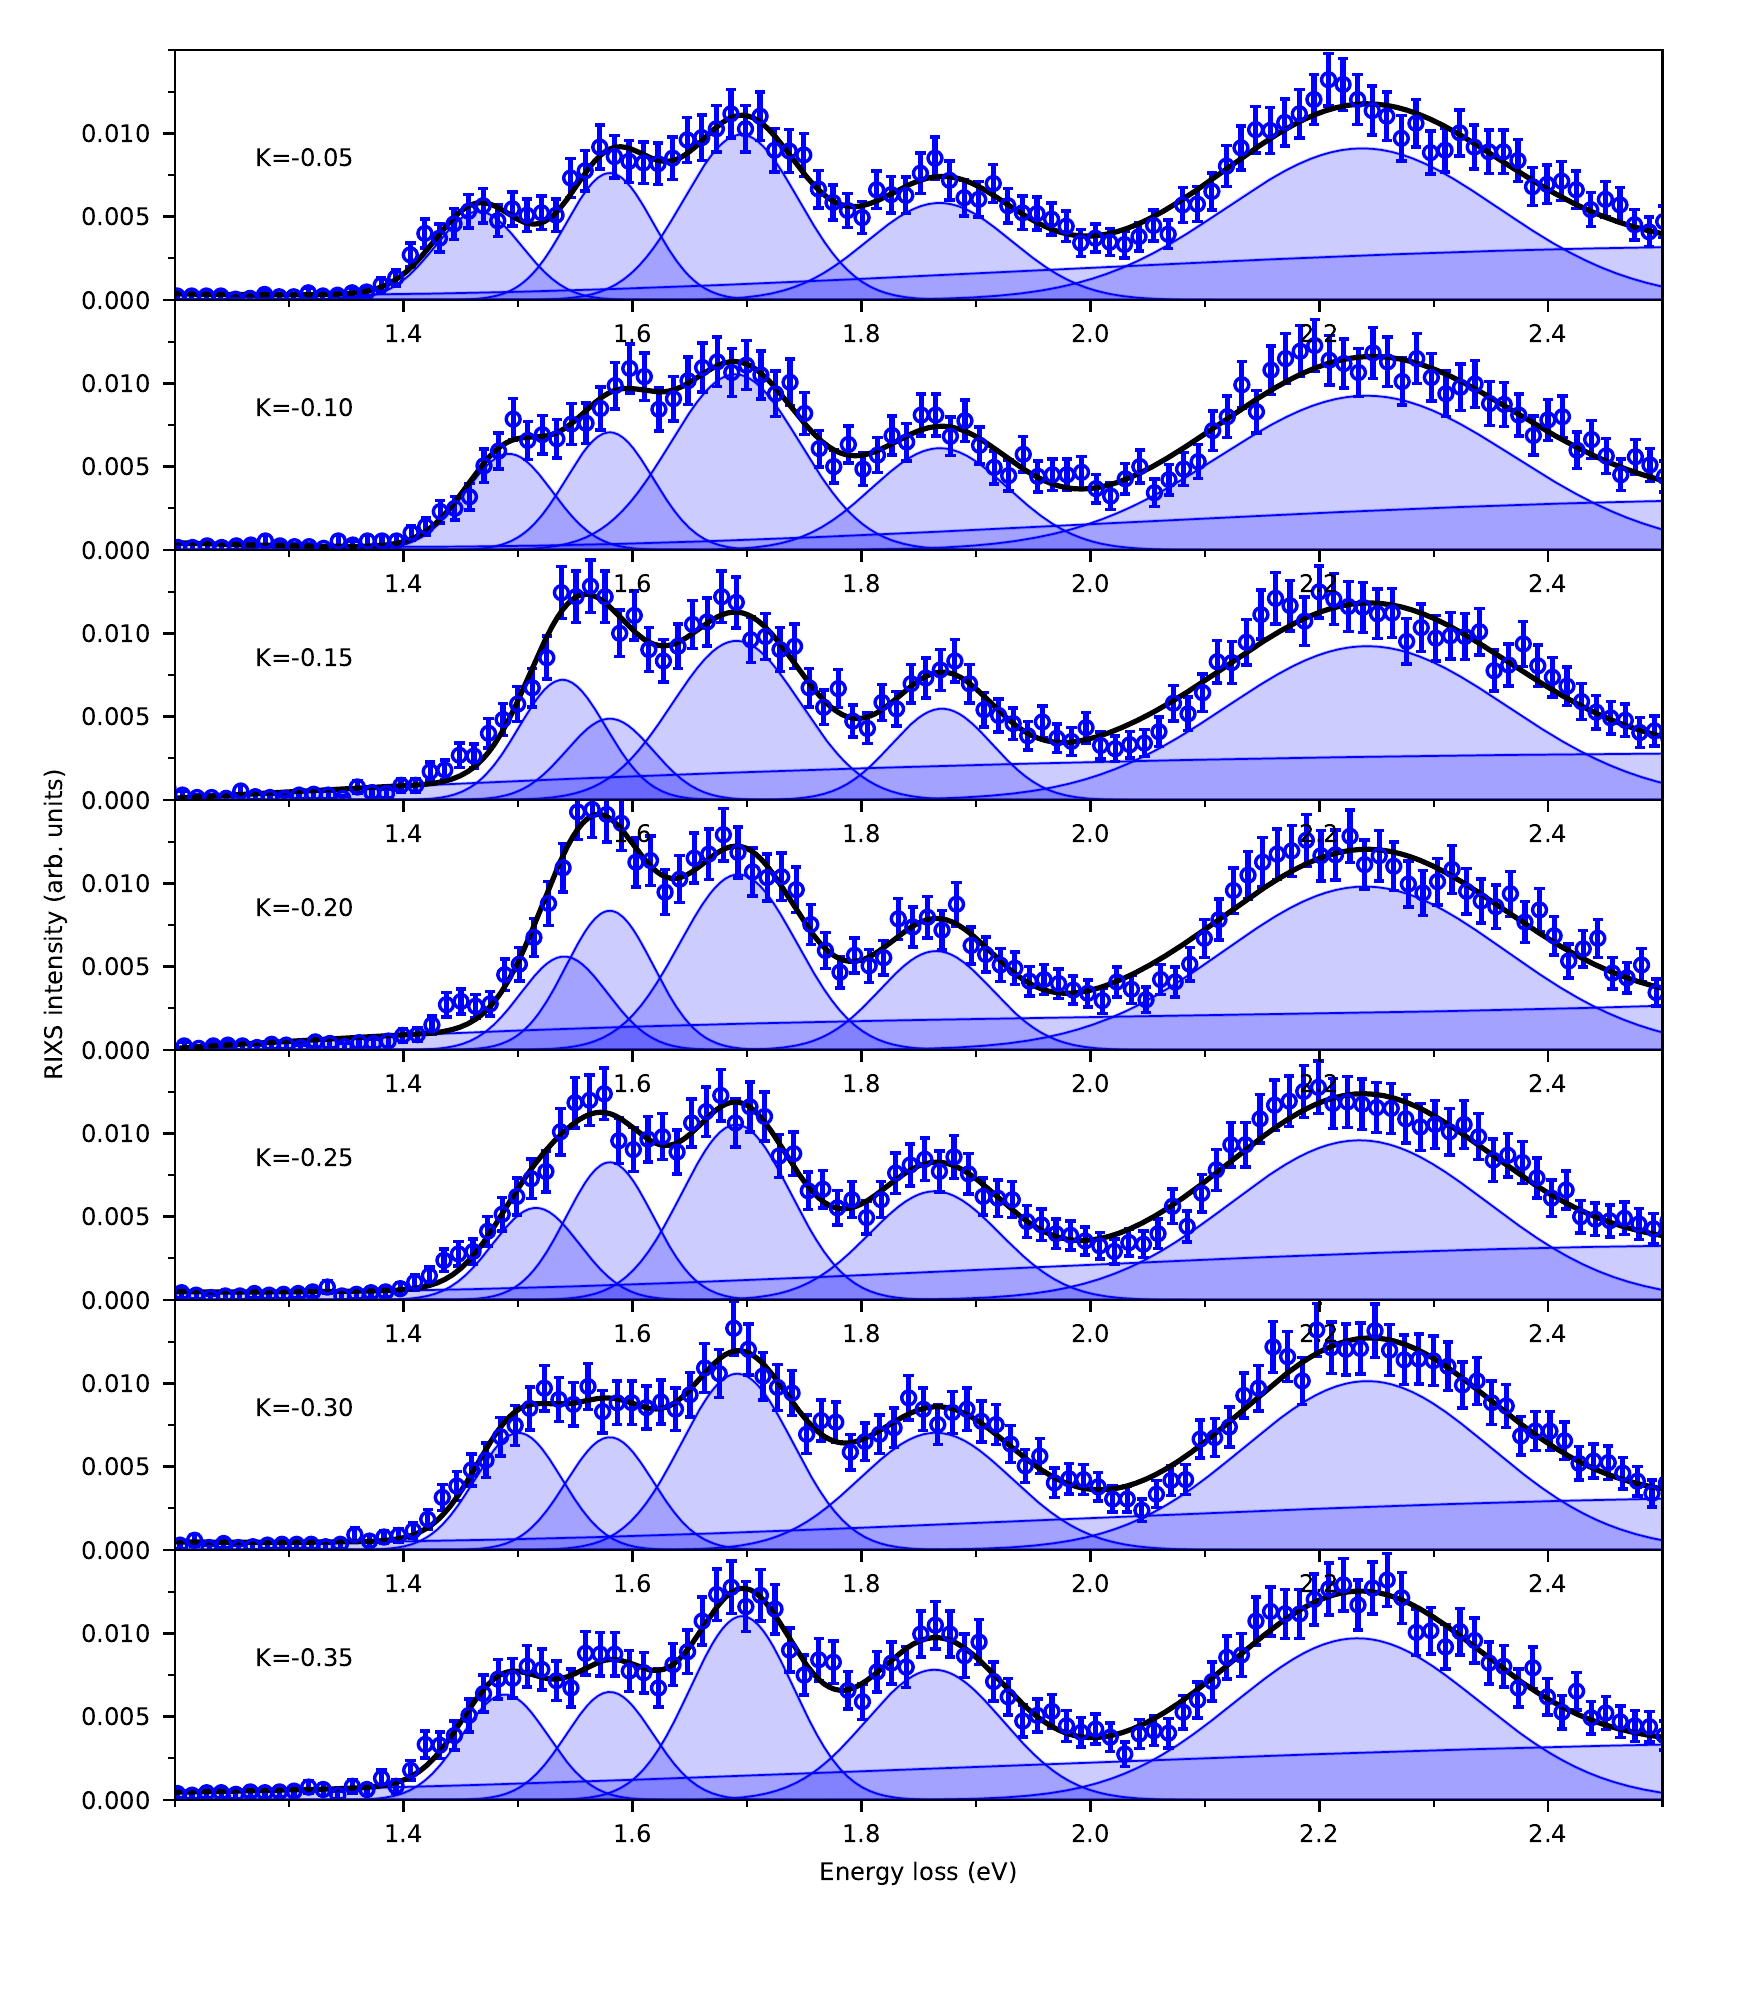}
    \caption{Fits to the spectra in the $0KL$ plane.}
    \label{fig:fits1}
\end{figure*}

\begin{figure*}[htb!]
    \centering
    \includegraphics[width=0.9\textwidth]{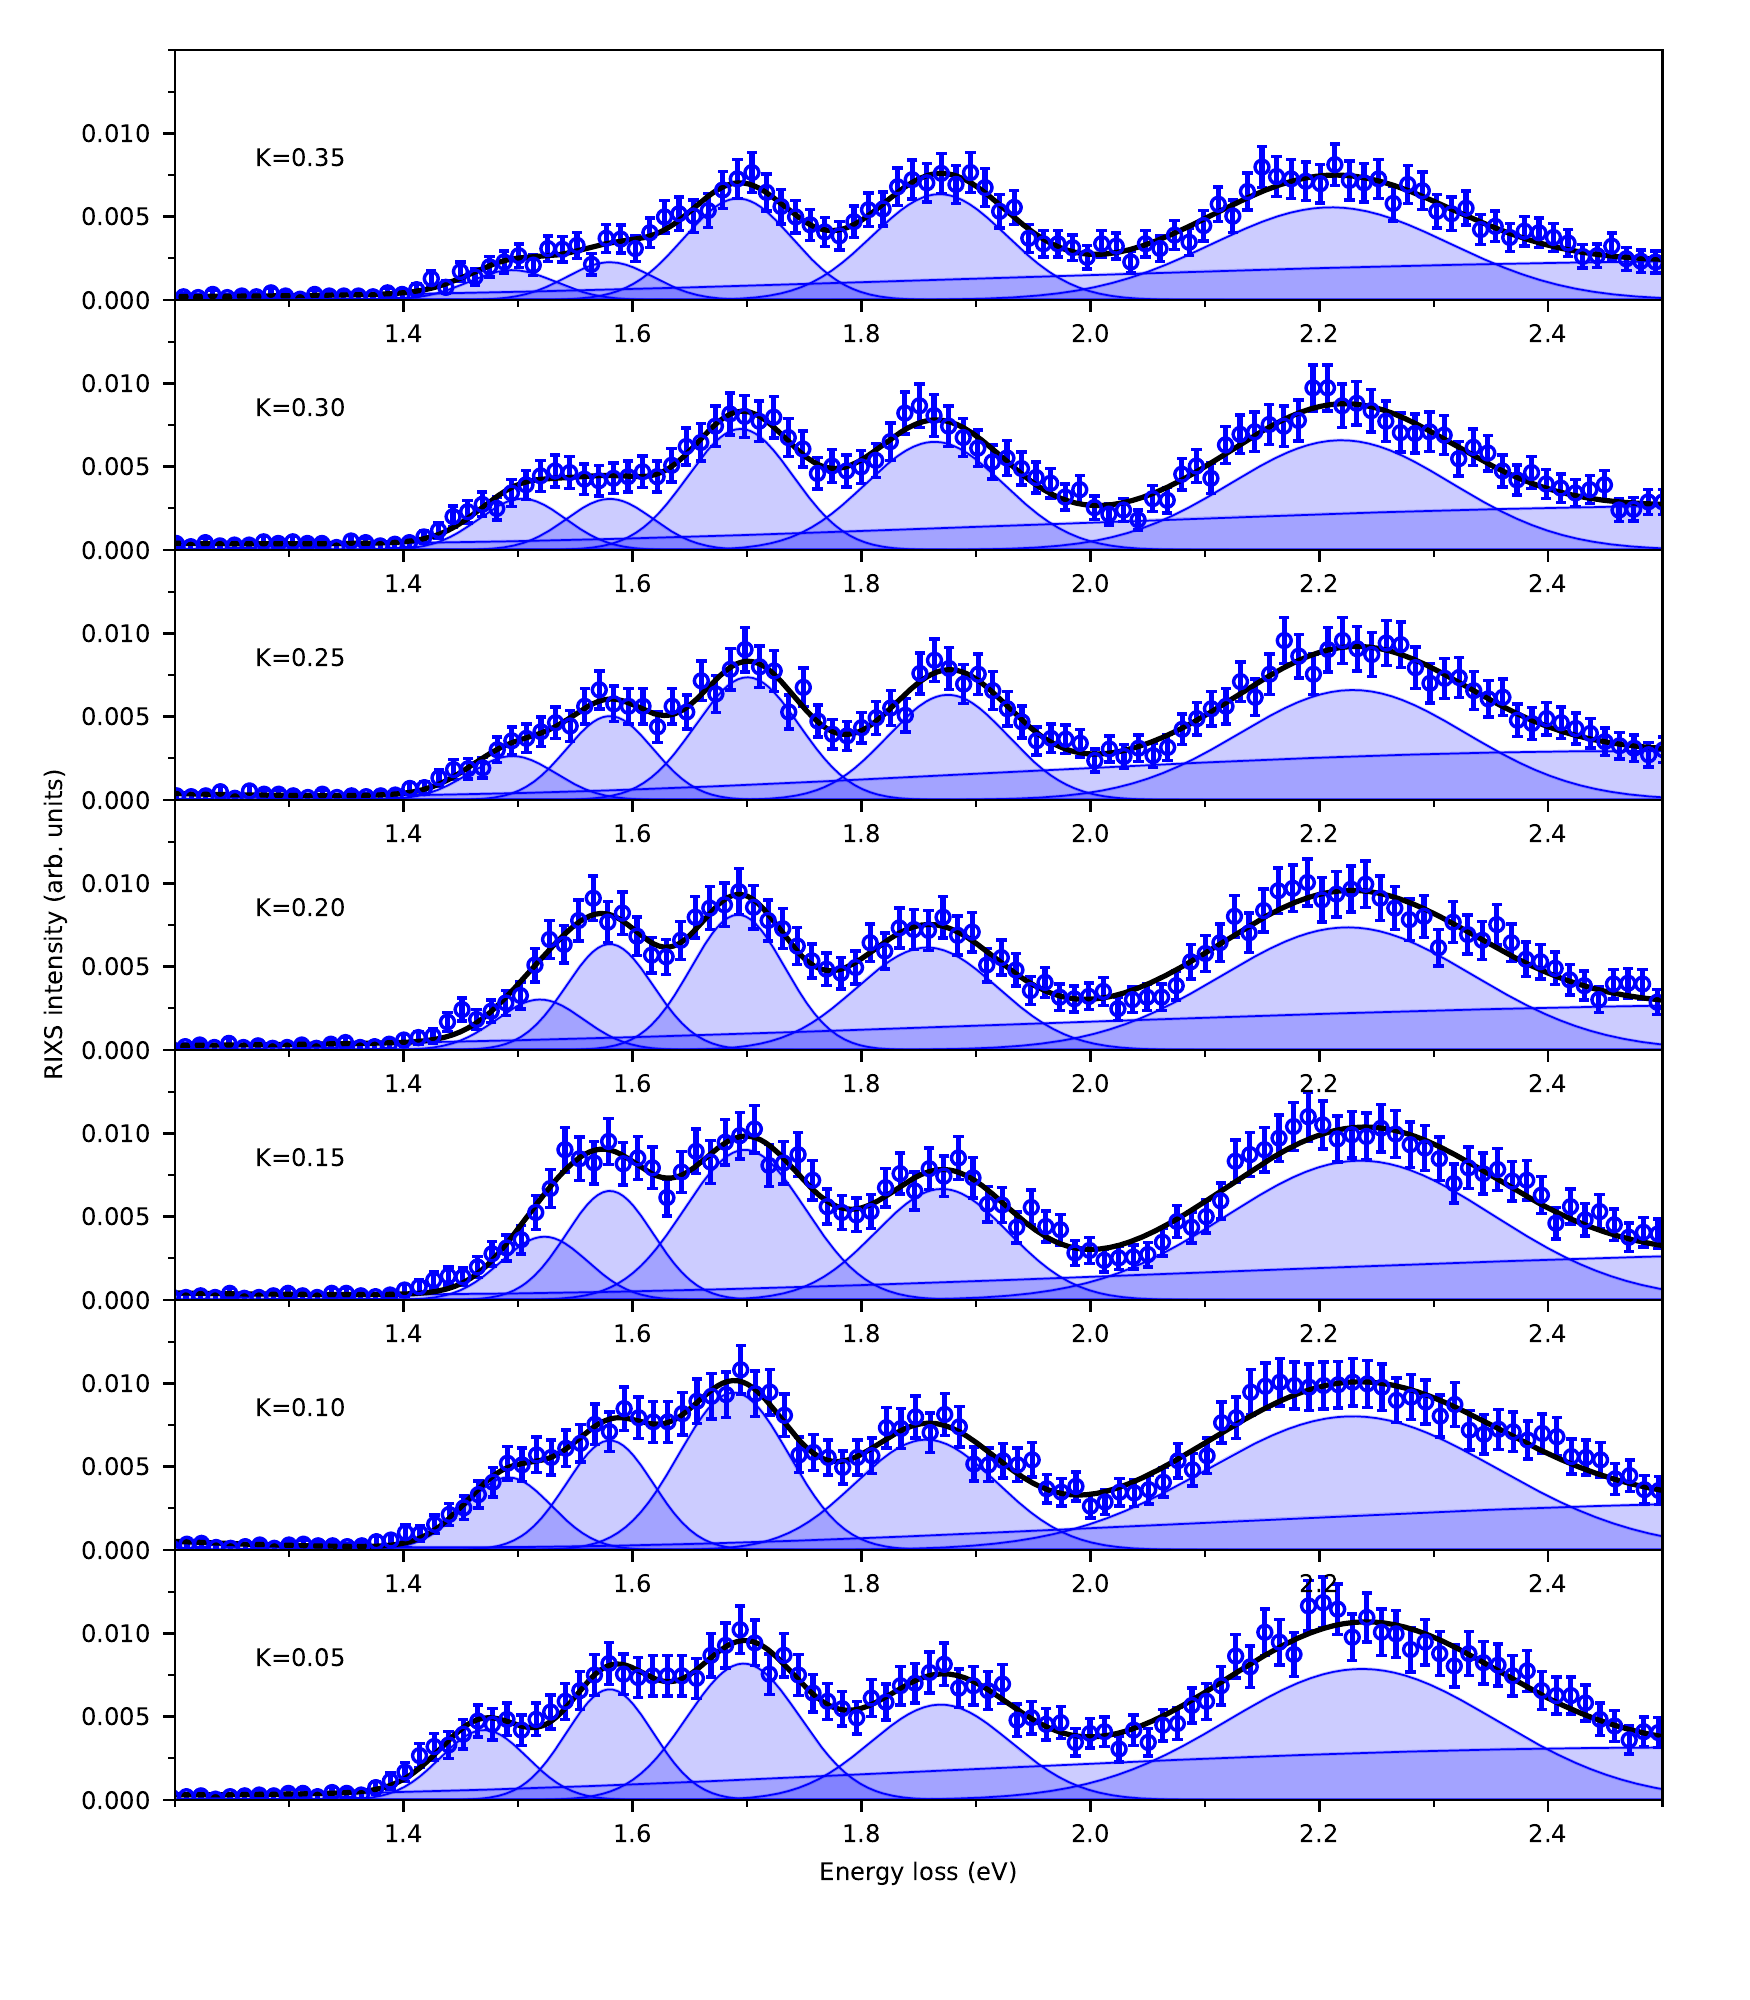}
    \caption{Fits to the spectra in the $0KL$ plane.}
    \label{fig:fits1}
\end{figure*}

\bibliography{refs}

\end{document}
